# Supplementary material for: Exploiting network information to disentangle spillover effects in a field experiment on teens' museum attendance
Source: arXiv:2011.11023 ancillary file (2022-05-06)
Supplement: Supplementary file 1 [file Appendix.pdf]

# Online Appendix for Exploiting Network Information to Disentangle Spillover Effects in a Field Experiment on Teens' Museum Attendance

## Identification Issues

If the compliance status were fully observed for each unit, under Assumptions ?? and ??, we could identify principal controlled direct and spillover effects using the following relationship between the conditional mean of the potential outcomes, $Y_{ij}(z, s_{\mathcal{N}_{ij}})$, given principal stratum membership and covariates and the conditional mean of the observed outcomes, $Y_{ij}$, given principal stratum membership, encouragement status, mediator and covariates:

$$E\left[Y_{ij}(z, s_{\mathcal{N}_{ij}}) \mid G_{ij} = g, \mathbf{X}_{ij}\right] = E\left[Y_{ij} \mid Z_j = z, S_{\mathcal{N}_{ij}} = s_{\mathcal{N}_{ij}}, G_{ij} = g, \mathbf{X}_{ij}\right] \tag{1}$$

Under Assumptions ??, ?? and ??, we could identify principal natural direct and indirect effects using the mediation formula (?):

$$\begin{aligned} &E\left[Y_{ij}(z, S_{\mathcal{N}_{ij}}(z')) \mid G_{ij} = g, \mathbf{X}_{ij}\right] = \\ &\int E\left[Y_{ij} \mid Z_j = z, S_{\mathcal{N}_{ij}} = s_{\mathcal{N}_{ij}}, G_{ij} = g, \mathbf{X}_{ij}\right] f_{S_{ij}}(s_{\mathcal{N}_{ij}} \mid Z_j = z', G_{ij} = g, \mathbf{X}_{ij}) \end{aligned} \tag{2}$$

Because the compliance status is only partially observed, we cannot directly use these relationships.

# Bayesian Inference

Under the assumption that the probabilities of extra zeros with respect to the Poisson distribution, $\phi_{ij,g,z}$, depend on the encouragement and the principal stratum membership, but not on covariates: $\phi_{ij,g,z} = \phi_{g,z}$, and the prior equalities of the slope coefficients and the standard deviations of the random intercepts in the Poisson regressions described described in the main text, the full parameter vector is $\boldsymbol{\theta} = \{\ (\gamma_g, \boldsymbol{\delta}_g; g \in \{000, 001, 011\}),\ \sigma_a,\ \phi_{000,1},\ \phi_{000,2} = \phi_{000,3},\ \phi_{001,1},\ \phi_{001,2},\ \phi_{001,3},\ \phi_{011,1},\ \phi_{011,2} = \phi_{011,3},\ \phi_{111,1},\ \phi_{111,2} = \phi_{111,3},\ \beta_1^{(S)},\ \beta_{000,2}^{(S)} = \beta_{000,3}^{(S)} = \beta_{001,2}^{(S)} = \beta_{011,2}^{(S)} = \beta_{011,3}^{(S)} = \beta_{111,2}^{(S)} = \beta_{111,3}^{(S)} = \beta_2^{(S)},\ \beta_{001,3}^{(S)},\ \boldsymbol{\beta}^{(X)},\ \sigma_b\}$ for a total of $3 \times (1+6) + 1 + 12 + 5 + 1 = 40$ parameters.

## Likelihood

Define $\pi_{ij}^{m_1m_2m_3} \equiv Pr\left(G_{ij} = m_1m_2m_3 \mid \boldsymbol{X}_{ij}, \boldsymbol{\theta}\right)$ and $f_{ij,z}^{m_1m_2m_3}(y) \equiv Pr\big(Y_{ij}(z, S_{\mathcal{N}_{ij}}(z)) = y \mid G_{ij} = m_1m_2m_3, \boldsymbol{X}_{ij}, \boldsymbol{\theta}\big)$. The observed data likelihood results in the following finite mixture model likelihood:

$$
\begin{aligned}
&\mathcal{L}(\boldsymbol{\theta} \mid \boldsymbol{Z}, \boldsymbol{C}, \boldsymbol{M}, \boldsymbol{Y}, \boldsymbol{X}) = \\
&\prod_{j:Z_j=1}\left[\prod_{i:C_{ij}=1,M_{ij}=0}\Big[\ \pi_{ij}^{011}\cdot f_{ij,1}^{011}(Y_{ij}) + \pi_{ij}^{001}\cdot f_{ij,1}^{001}(Y_{ij}) + \pi_{ij}^{000}\cdot f_{ij,1}^{000}(Y_{ij})\Big] \times \prod_{i:C_{ij}=1,M_{ij}=1}\pi_{ij}^{111}\cdot f_{ij,1}^{111}(Y_{ij})\right] \times \\
&\prod_{j:Z_j=2}\left[\prod_{i:C_{ij}=1,M_{ij}=0}\Big[\pi_{ij}^{001}\cdot f_{ij,1}^{001}(Y_{ij}) + \pi_{ij}^{000}\cdot f_{ij,1}^{000}(Y_{ij})\Big] \times \prod_{i:C_{ij}=1,M_{ij}=1}\Big[\pi_{ij}^{111}\cdot f_{ij,1}^{111}(Y_{ij}) + \pi_{ij}^{011}\cdot f_{ij,1}^{011}(Y_{ij})\Big]\right] \times \\
&\prod_{j:Z_j=3}\left[\prod_{i:C_{ij}=1,M_{ij}=0}\pi_{ij}^{000}\cdot f_{ij,1}^{000}(Y_{ij}) \times \prod_{i:C_{ij}=1,M_{ij}=1}\Big[\big(\pi_{ij}^{111}\cdot f_{ij,1}^{111}(Y_{ij}) + \pi_{ij}^{011}\cdot f_{ij,1}^{011}(Y_{ij}) + \pi_{ij}^{001}\cdot f_{ij,1}^{001}(Y_{ij})\Big]\right]
\end{aligned}
$$

where $\boldsymbol{Z}$ is a $J-$ dimensional vector with $jth$ element equal to $Z_j$, $\boldsymbol{C}, \boldsymbol{M}$, and $\boldsymbol{Y}$ are $N-$ dimensional vectors with $ijth$ elements equal to $C_{ij}$, $M_{ij}$ and $Y_{ij}$, respectively, and $\boldsymbol{X}$ is an $N \times K$ matrix with $ij$th row equal to $\boldsymbol{X}_{ij}$, $i = 1, \ldots, N_j$, $j = 1, \ldots, J$.

Let $p(\boldsymbol{\theta})$ denote the joint prior distribution of $\boldsymbol{\theta}$. The posterior distribution,

$$p(\boldsymbol{\theta} \mid \boldsymbol{Z}, \boldsymbol{C}, \boldsymbol{M}, \boldsymbol{Y}, \boldsymbol{X}) \propto p(\boldsymbol{\theta}) \times \mathcal{L}(\boldsymbol{\theta} \mid \boldsymbol{Z}, \boldsymbol{C}, \boldsymbol{M}, \boldsymbol{Y}, \boldsymbol{X})$$

is analytically intractable due to the complex mixture structure of the likelihood function. We deal with computational issues approximating the posterior distribution via Stan, a Bayesian programming language that implements a variant of Hamiltonian Monte Carlo (**?**).

## Priors specification

We assume that the parameters are a priori independent and specify relative weakly informative prior distributions for them. Specifically, we postulate independent normal priors with prior mean equal to 0 and standard deviations equal to 2.5 for the coefficients of the principal strata model, $\gamma_g$ and $\boldsymbol{\delta}_g$, and independent normal priors with prior mean equal to 0 and standard deviations equal to 1 for the coefficients of the potential outcome models, $\alpha_{g,z}$, $\beta^{(S)}_{g,z}$ and $\boldsymbol{\beta}^{(X)}$. Finally, we specify half-normal prior distributions with a standard deviation equal to 0.5 for the standard deviations $\sigma_a$ and $\sigma_b$ of the random intercepts $a_j$ and $b_j$, entering the principal strata model and the potential outcome models (**?**). The choice of the values of the parameters of the prior distributions, in general, and of the standard deviations of the Normal priors was partially driven by stability issues arising from running the algorithm we use to derive the posterior distribution.

## Estimation of the effects

For the estimation of finite population principal causal effects we adopt an imputation approach. At each iteration, for each unit missing potential outcomes for $Y_{ij}$ and $M_{ij}$ are imputed using their predictive posterior distribution. Then, overall average principal causal effects are computed as function of the observed and missing information. For calculate principal controlled direct and spillover effects, under Assumption **??**, we use Equation 1 condi-

tionally on the imputed principal stratum membership. Specifically we impute $Y_{ij}(z, s_{\mathcal{N}_{ij}})$ for all units using the potential outcome models in Equation **??** and average over the empirical distribution of the covariates in each principal stratum. Similarly to calculate principal natural direct and indirect effects we first calculate the missing potential outcomes for the proportion of friends visiting palazzo vecchio in the first place, $S_{\mathcal{N}_{ij}}$, using the observed and imputed values for $M_{ij}$. Then, under Assumptions **??** and **??**, we use Equation 2 conditionally on the imputed principal stratum membership.
